# Supplementary material for: Contrastive Deep Encoding Enables Uncertainty-aware Machine-learning-assisted Histopathology
Source: arXiv:2309.07113 source file (2023-09-13)
Supplement: Supplementary file 1 [file supp.tex]

% Template for ICASSP-2021 paper; to be used with:
%          spconf.sty  - ICASSP/ICIP LaTeX style file, and
%          IEEEbib.bst - IEEE bibliography style file.
% --------------------------------------------------------------------------
\documentclass{article}
\usepackage{spconf,amsmath,graphicx}
\usepackage{threeparttable}
\usepackage{amsfonts}
 % Arial
%\renewcommand{\sfdefault}{phv} % Arial

\usepackage{multirow}
\usepackage{cite}
\usepackage{svg}
\usepackage{url}
\usepackage{xcolor}

\usepackage{hyperref}

\usepackage{graphicx}
\usepackage{textcomp}
\usepackage{xcolor}
\usepackage{comment}
\usepackage{blindtext}
\usepackage{siunitx}
\usepackage{graphicx}
\usepackage{subcaption}
\usepackage{balance}
\usepackage{bm}
\usepackage{multirow}
\usepackage{booktabs}
\usepackage{pifont}% http://ctan.org/pkg/pifont
\usepackage[linesnumbered,ruled,vlined]{algorithm2e}

% \hypersetup{
%     colorlinks=true, %set true if you want colored links
%     linktoc=all,     %set to all if you want both sections and subsections linked
%     linkcolor=black,  %choose some color if you want links to stand out
%     }

% Example definitions.
% --------------------

% Title.
% ------
\title{Supplementary Materials for Deep Encoding for Machine Learning Assisted Histopathology}
\begin{document}

\maketitle
\input{Sections/Appendix}

\end{document}
